# Supplementary material for: CRoF: CLIP-based Robust Few-shot Learning on Noisy Labels
Source: arXiv:2412.12793 source file (2024-12-17)
Supplement: Supplementary file 1 [file X_suppl.tex]

\clearpage
\setcounter{page}{1}
\maketitlesupplementary

\section{Discussion of Multiple Label Weighting}

In this section, we provide supplementary analysis on the multiple label weighting, focusing on the effectiveness of gradient updating and model optimization.

\subsection{Gradient Analysis}
The loss function of each sample in our proposals is in \cref{eq:losss}, where $y_i$ is the one-hot hard label.
$w_i^*$ indicates the contribution of the highly similar labels.
 $p_i$ is the prediction by softmax and $z_i$ is the logits.
 The gradient is calculated by \cref{eq:gradient}.

In scenario 1, both $w_1$  and $s_1$ are the largest, so $w_1^*$=1 according to \cref{eq:7}. Here, \cref{eq:losss} simplifies to the standard cross-entropy loss function. 

In scenario 2, the weights of the original and the most similar labels, $w_r^*$ and $w_1^*$,  are larger than those of the other labels, which both consider the similarity rank and the influence of the hyper-parameters.
Therefore,  $w_r^*$ and $w_1^*$ contribute to a greater gradient.
For the remaining $K$-2 candidates labels, the smaller weights $w_i^*$ help reduce the interference to the overall gradient.

In scenario 3, the original label is not considered to be ground truth and is discarded. 
The weights of \textit{top-K} labels are determined by hyperparameter \( \beta \) to balance the most similar label and others. So $w_1^*$ is the largest, contributing significantly to the model training with a greater gradient.

So, the weighting module achieves a specific smooth distribution of the ground truth class and other classes,  assigning reasonable contributions to the gradient in top-ranked classes.

\begin{equation}\label{eq:losss}
 L = -\sum_{i=1}^{K} w_i^* y_i \log p_i
\end{equation}

\begin{equation}\label{eq:gradient}
\frac{\partial L}{\partial z_i} = w_i^* \cdot (p_i - y_i)
\end{equation}

\subsection{Opitimization Analysis}

The weight distribution in our method is influenced by three hyper-parameters ($\alpha, \beta, \gamma$).
$\alpha$ represents the degree of loyalty to the original label, $\beta$ indicates the confidence to the most similar label, and $\gamma$ is the impact of ranking on weight  distribution.
Based on the assumption in  paper\cite{Szegedy_2016_CVPR}, it is better to set $\alpha, \beta, \gamma$ with a larger value.
This research proposes a fixed uniform distribution to the other label.
Consequently, the cross-entropy between the uniform distribution and prediction distribution acts as the regularization of the original cross-entropy, avoiding overfitting to the hard label.

Traditional label smoothing assigns fixed weights to all categories, which introduces extra noise information from irrelevant categories. 
In contrast, our proposal confines the weight distribution to the $top-K$ most similar categories, allowing the model to make more robust predictions for boundary categories.
Our method not only retains the advantages of label smoothing in mitigating overfitting but also minimizes the impact of noise from irrelevant categories.

The ranking $r$ of the original label in the $S^*$ also plays a crucial role in balancing the $w_1$ and $w_r$ in \cref{eq:2}.
We assume that $w_r>w_1$, because the original label deserves more contribution.
Considering $S^*$, a larger $w_r$ would enhance the power of the smaller similarity of the original label.
If $w_r>w_1$, $r$  satisfies the condition in \cref{eq:r}. 
The maximal $K$ is also calculated in \cref{eq:r}. 
% If $r\leq K$, $w_r>w_1$.

\begin{equation}\label{eq:r}
\begin{split}
\alpha \cdot \gamma^{r-2} & > (1-\alpha \cdot \gamma^{r-2}) \cdot \beta \\
r & < 2 + \frac{\ln\left(\frac{\beta}{\alpha(1+\beta)}\right)}{\ln(\gamma)}  
\end{split}
\end{equation}

\section{Prompt Analysis}
We have completed the prompt analysis for the nine datasets listed in the submission manuscript. Only two of them are presented in the main text for limited space and more comprehensive experimental results are presented here.

\subsection{Similarity Heatmap}

In the supplementary material, we present the heatmaps of embeddings for different prompts in \cref{fig:Heatmap1} and \cref{fig:Heatmap2}, apart from $UCF101$ and $Caltech101$ listed in the submission manuscript.
\cref{fig:Heatmap1} illustrates the performance of prompts on the fine-grained image reognition task datasets.
In \cref{fig:Heatmap2}, we show three recognition tasks: scene recognition,  generic object recognition and texture classification. 

 After applying our method, the inter-class similarity has decreased in most cases.
Sup prompt increases the distance of label embedding and introduces more noisy information, such as on $Flowers102$.
TPG, combining the Sup and CaFo, achieves a balanced distance between the categories, which is larger than CaFo but smaller than Sup.
Besides, the similarity distribution varies on different datasets. 
For example, the similarity in $DTD$ is larger than that of other datasets on average.
Even in such cases, Sup prompt and TPG still increase the distance.
  The comprehensive experiments prove that our prompt method reduces the similarity and gives more tolerance to noisy labels.

\begin{figure*}[t]
    \centering

    \begin{subfigure}{0.22\linewidth}
        \centering
        \includegraphics[width=\linewidth, height=0.57\linewidth]{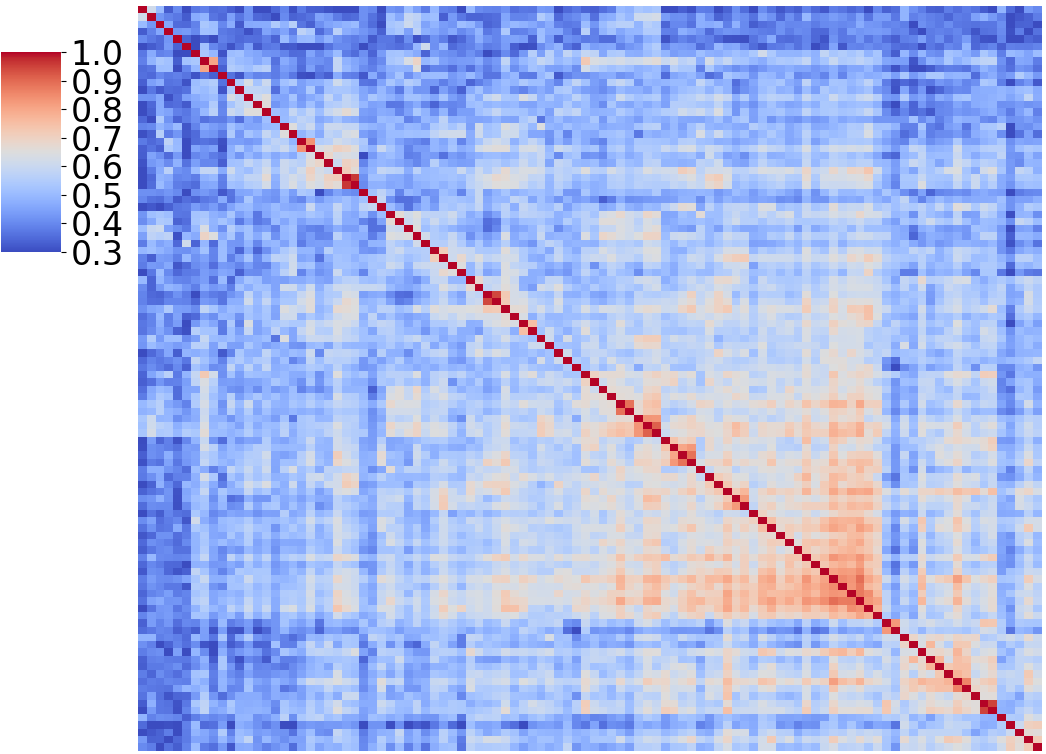}
        \caption{Org on \textit{Flowers102}}
        \label{fig:Flowers102org}
    \end{subfigure}
    \hspace{0.001\linewidth} % 控制水平间隔
    \begin{subfigure}{0.22\linewidth}
        \centering
        \includegraphics[width=\linewidth, height=0.57\linewidth]{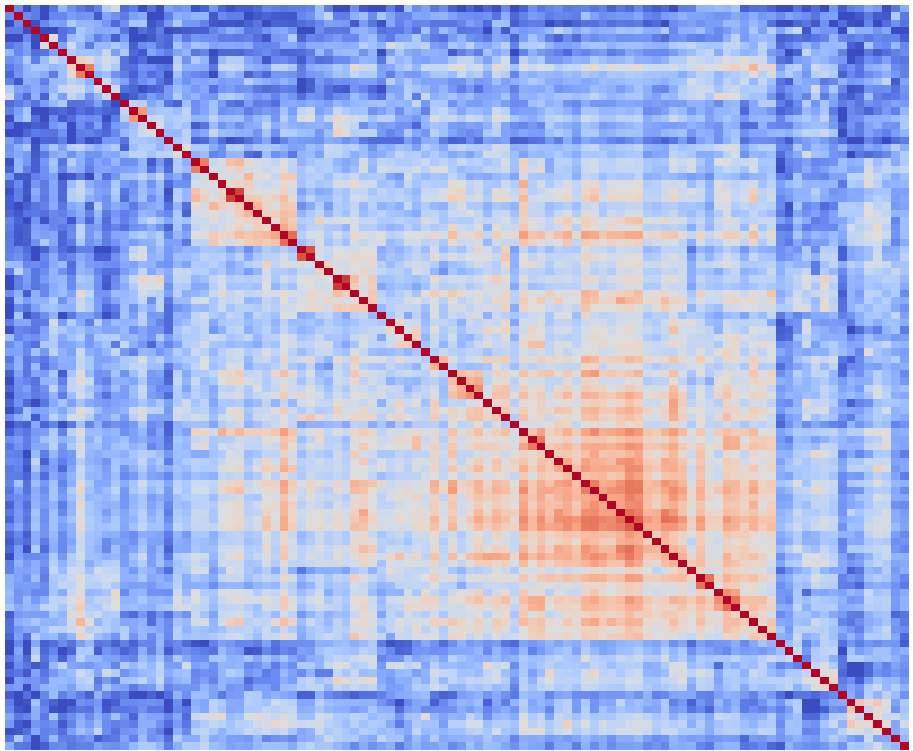}
        \caption{CaFo on \textit{Flowers102}}
        \label{fig:Flowers102cafo}
    \end{subfigure}        
    \hspace{0.001\linewidth} % 控制水平间隔
    \begin{subfigure}{0.22\linewidth}
        \centering
        \includegraphics[width=\linewidth, height=0.57\linewidth]{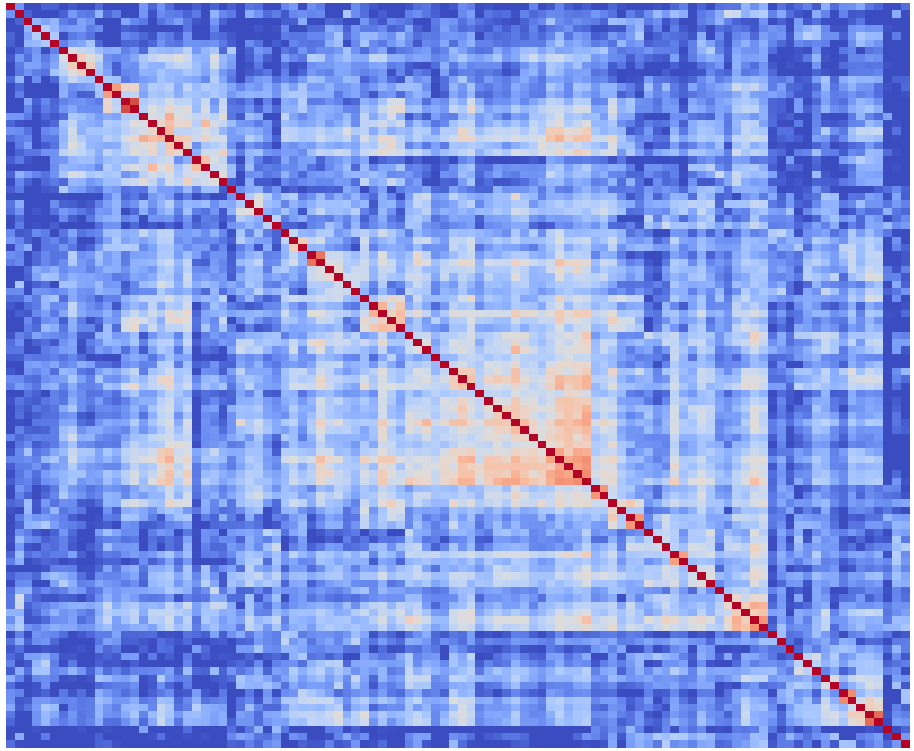}
        \caption{Sup on \textit{Flowers102}}
        \label{fig:Flowers102mine}
    \end{subfigure}    
    \hspace{0.001\linewidth} % 控制水平间隔
    \begin{subfigure}{0.22\linewidth}
        \centering
        \includegraphics[width=\linewidth, height=0.57\linewidth]{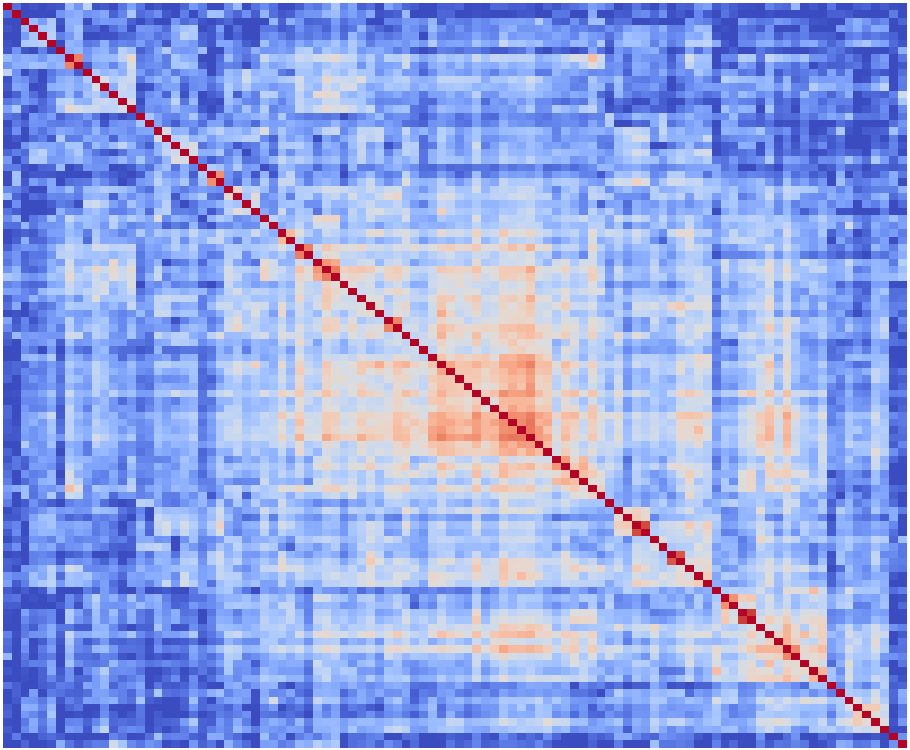}
        \caption{TPG on \textit{Flowers102}}
        \label{fig:Flowers102hunhe}
    \end{subfigure}

    % \vspace{0.1cm} % 控制垂直间隔

    \begin{subfigure}{0.22\linewidth}
        \centering
        \includegraphics[width=\linewidth, height=0.57\linewidth]{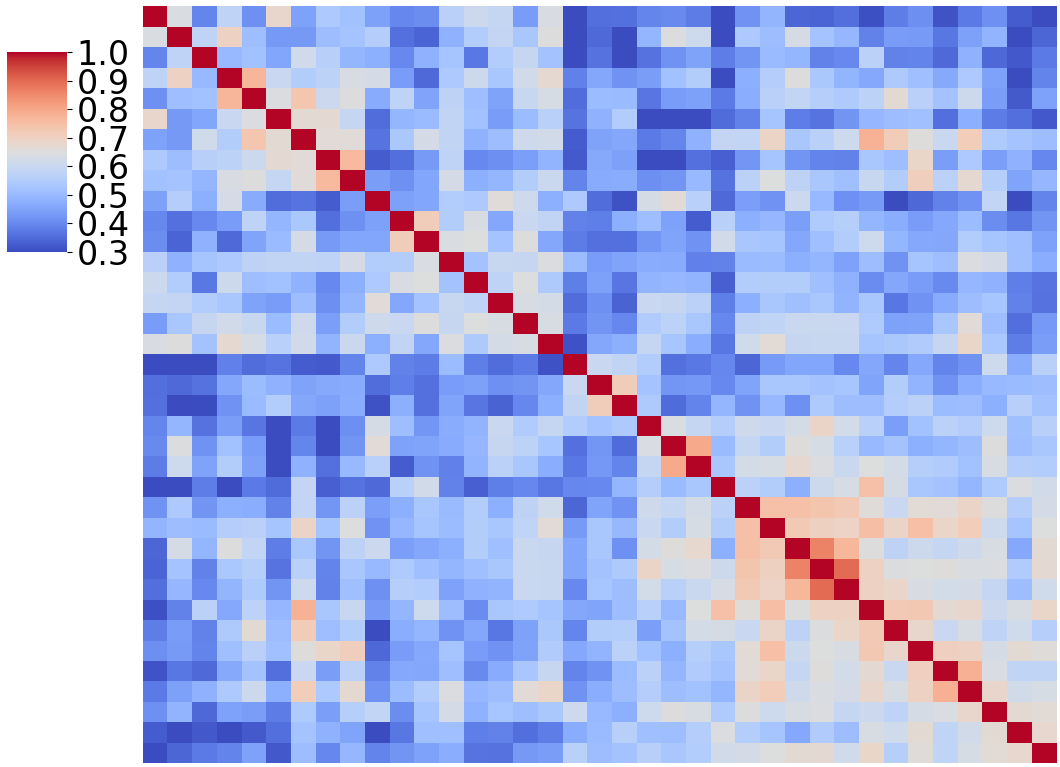}
        \caption{Org on \textit{OxfordPets}}
        \label{fig:OxfordPetsorg}
    \end{subfigure}
    \hspace{0.001\linewidth} % 控制水平间隔
    \begin{subfigure}{0.22\linewidth}
        \centering
        \includegraphics[width=\linewidth, height=0.57\linewidth]{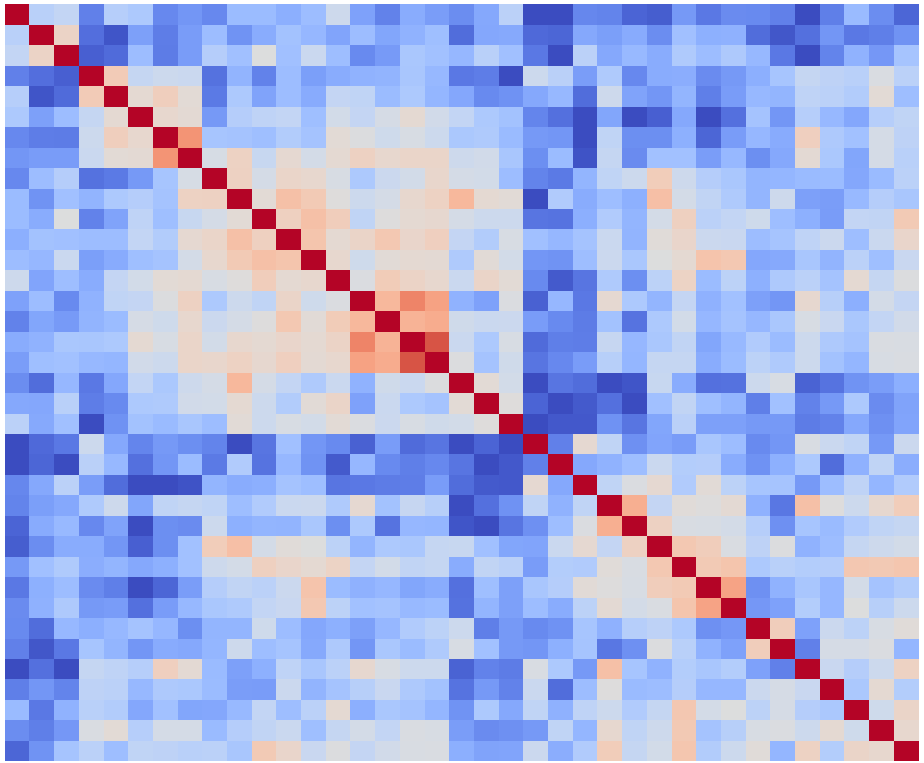}
        \caption{CaFo on \textit{OxfordPets}}
        \label{fig:OxfordPetscafo}
    \end{subfigure}        
    \hspace{0.001\linewidth} % 控制水平间隔
    \begin{subfigure}{0.22\linewidth}
        \centering
        \includegraphics[width=\linewidth, height=0.57\linewidth]{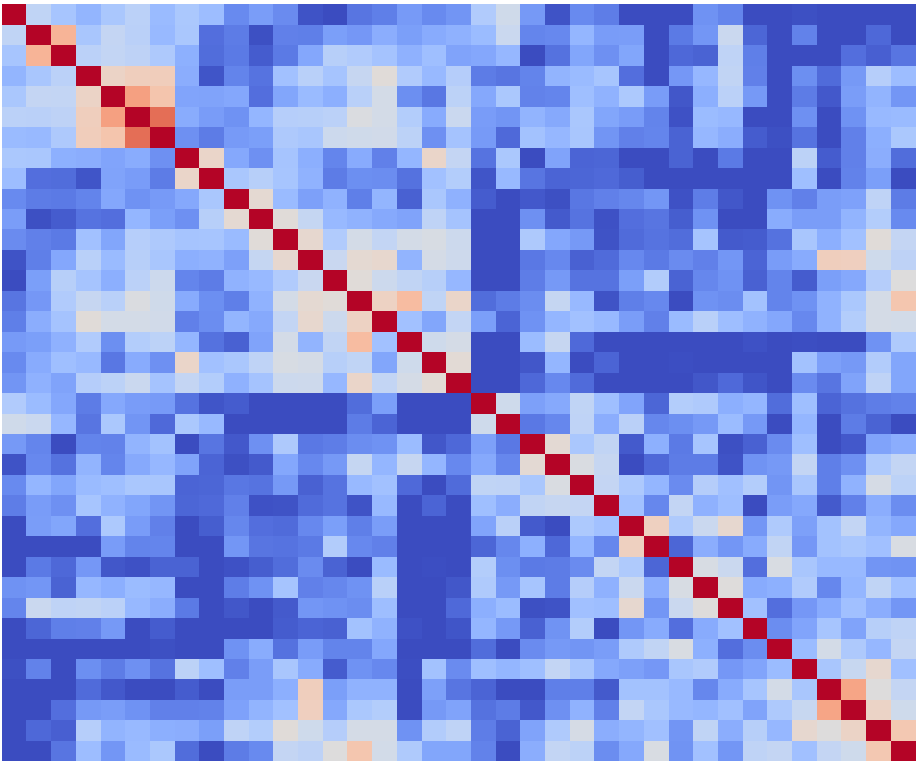}
        \caption{Sup on \textit{OxfordPets}}
        \label{fig:OxfordPetsmine}
    \end{subfigure}    
    \hspace{0.001\linewidth} % 控制水平间隔
    \begin{subfigure}{0.22\linewidth}
        \centering
        \includegraphics[width=\linewidth, height=0.57\linewidth]{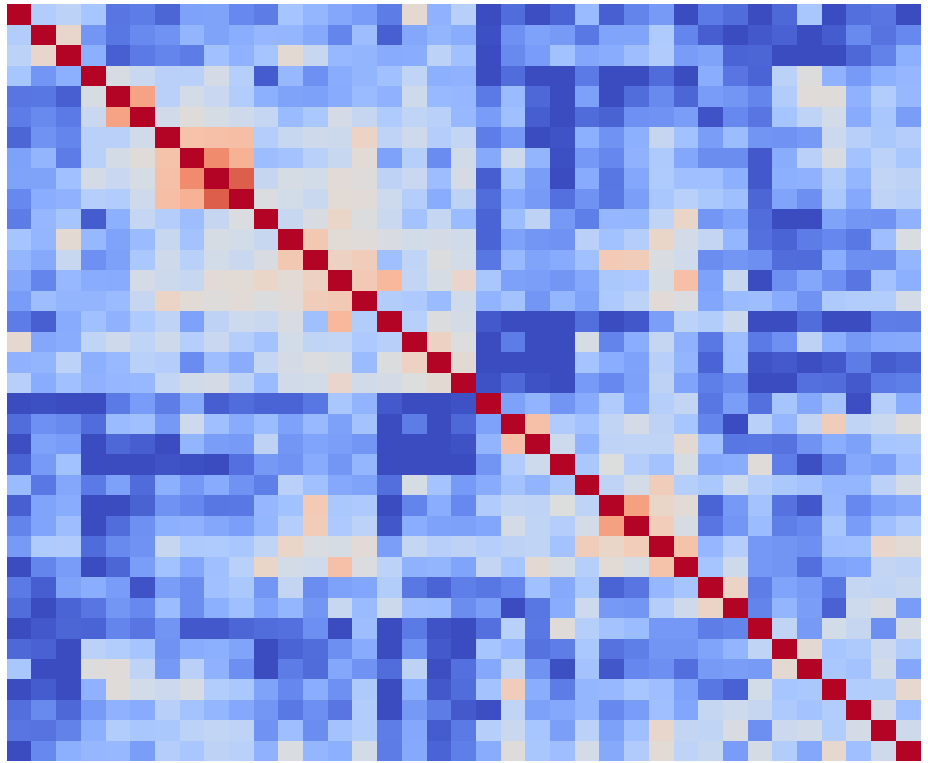}
        \caption{TPG on \textit{OxfordPets}}
        \label{fig:OxfordPetshunhe}
    \end{subfigure}
    % \vspace{0.1cm} % 控制垂直间隔
    
 \begin{subfigure}{0.22\linewidth}
        \centering
        \includegraphics[width=\linewidth, height=0.57\linewidth]{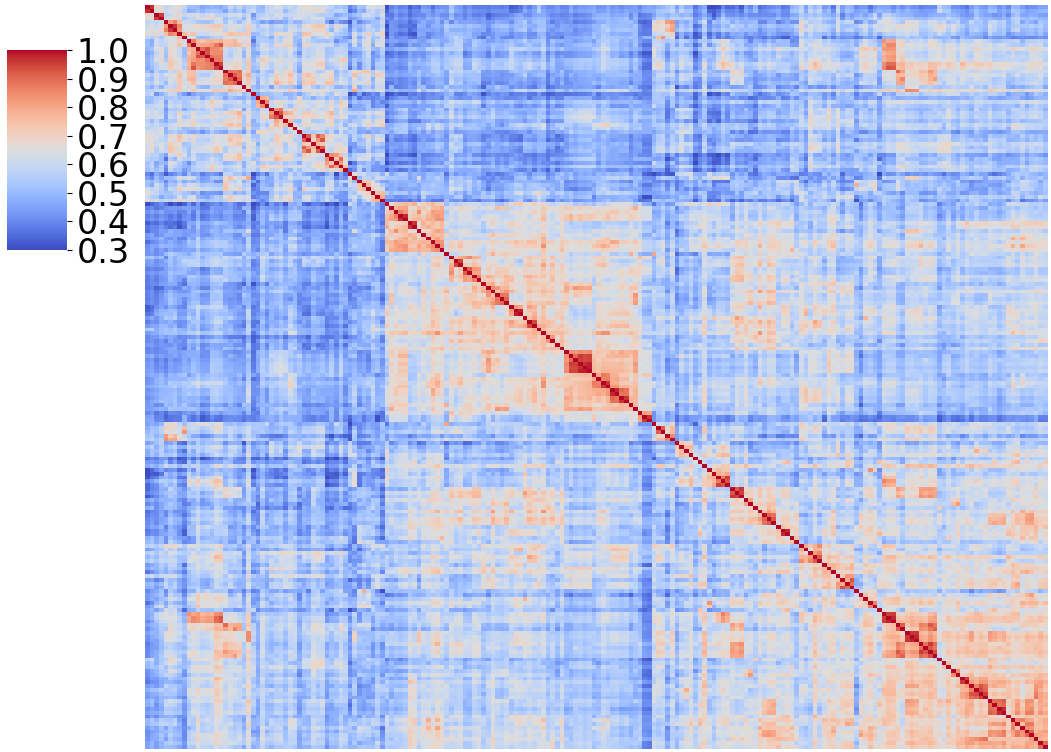}
        \caption{Org on \textit{StanfordCars}}
        \label{fig:StanfordCarsorg}
    \end{subfigure}
    \hspace{0.001\linewidth} % 控制水平间隔
    \begin{subfigure}{0.22\linewidth}
        \centering
        \includegraphics[width=\linewidth, height=0.57\linewidth]{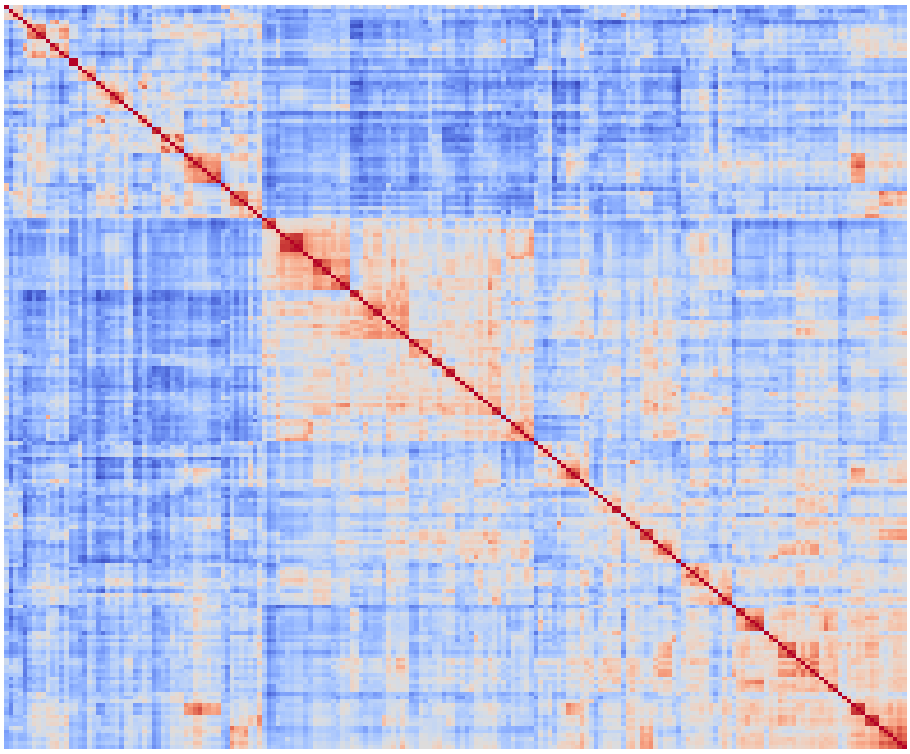}
        \caption{CaFo on \textit{StanfordCars}}
        \label{fig:StanfordCarscafo}
    \end{subfigure}        
    \hspace{0.001\linewidth} % 控制水平间隔
    \begin{subfigure}{0.22\linewidth}
        \centering
        \includegraphics[width=\linewidth, height=0.57\linewidth]{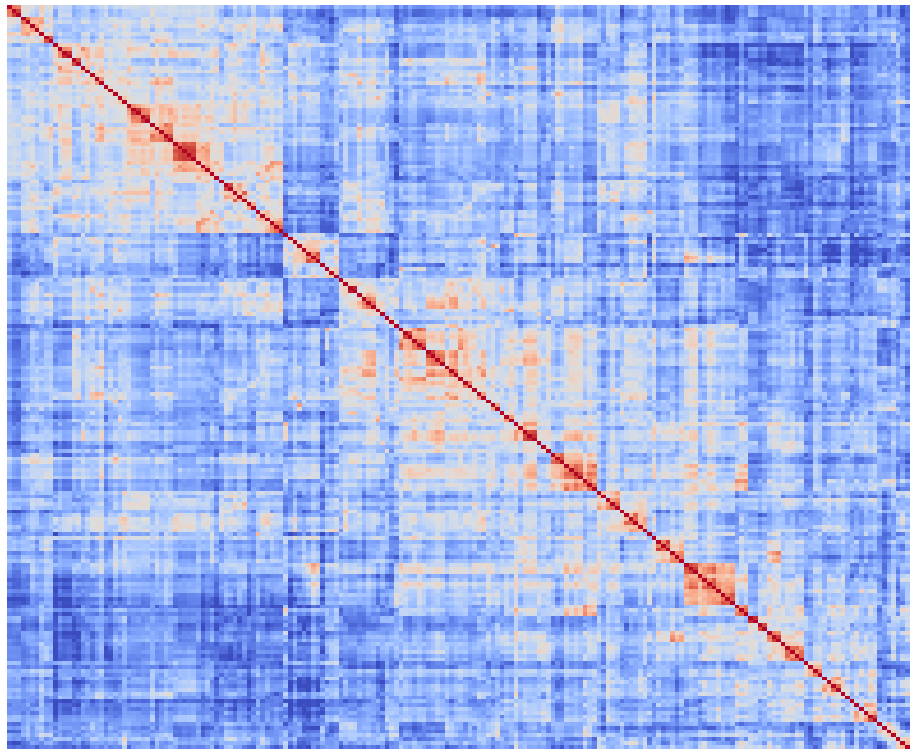}
        \caption{Sup on \textit{StanfordCars}}
        \label{fig:StanfordCarsmine}
    \end{subfigure}    
    \hspace{0.001\linewidth} % 控制水平间隔
    \begin{subfigure}{0.22\linewidth}
        \centering
        \includegraphics[width=\linewidth, height=0.57\linewidth]{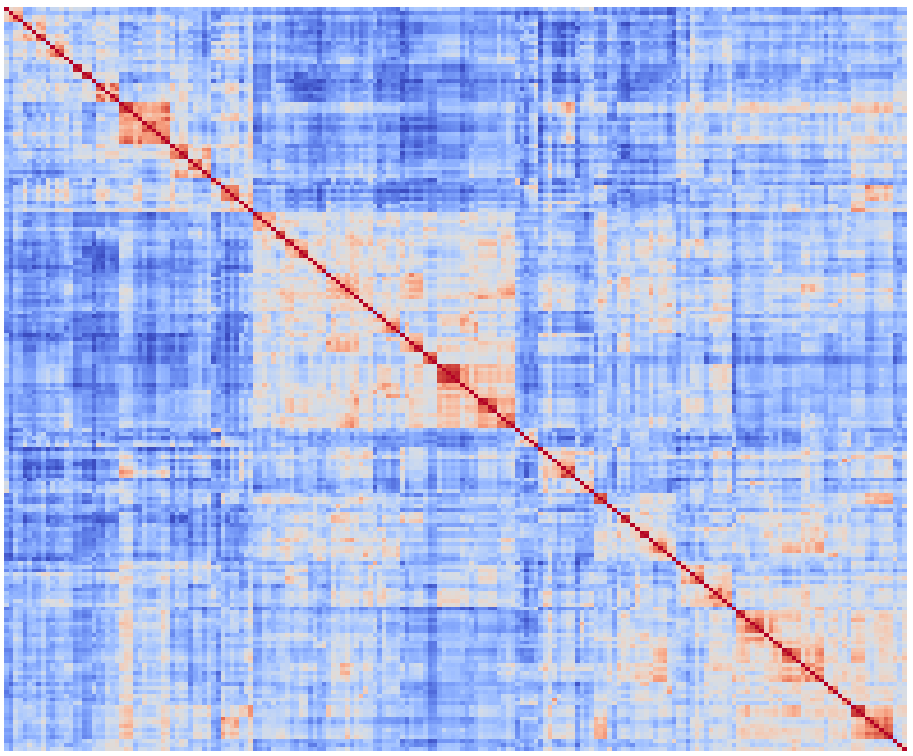}
        \caption{TPG on \textit{StanfordCars}}
        \label{fig:StanfordCarshunhe}
    \end{subfigure}

 %   
    % \vspace{0.1cm} % 控制垂直间隔
    \begin{subfigure}{0.22\linewidth}
        \centering
        \includegraphics[width=\linewidth, height=0.57\linewidth]{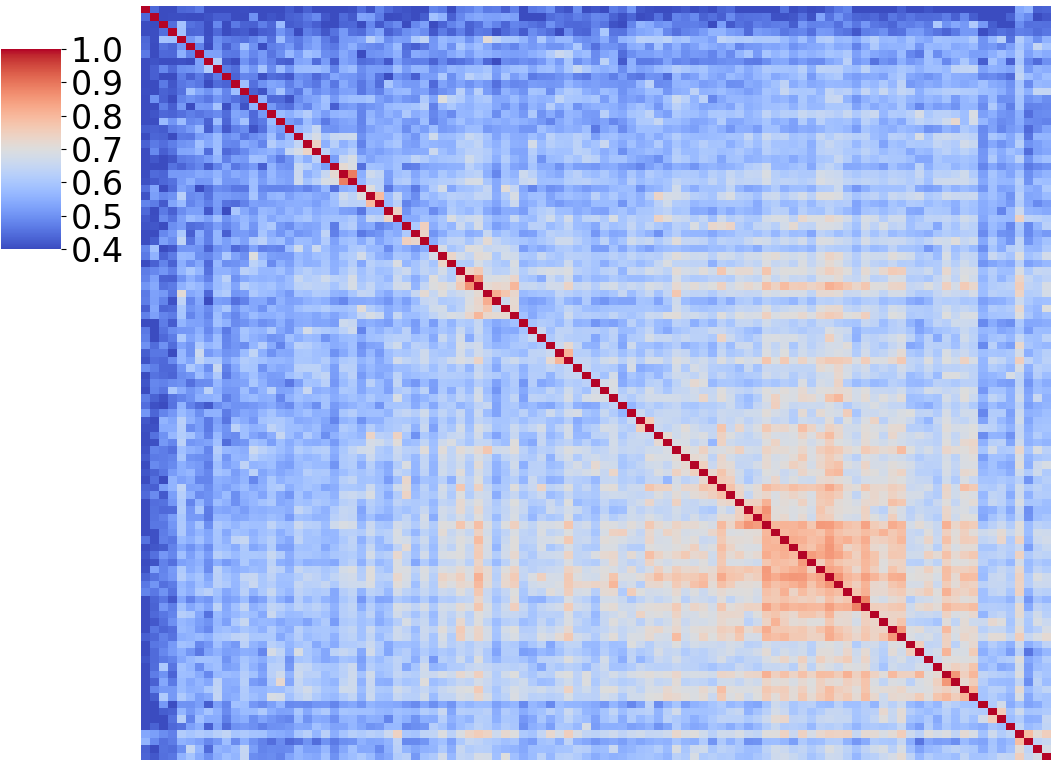}
        \caption{Org on \textit{Food101}}
        \label{fig:Food101org}
    \end{subfigure}
    \hspace{0.001\linewidth} % 控制水平间隔
    \begin{subfigure}{0.22\linewidth}
        \centering
        \includegraphics[width=\linewidth, height=0.57\linewidth]{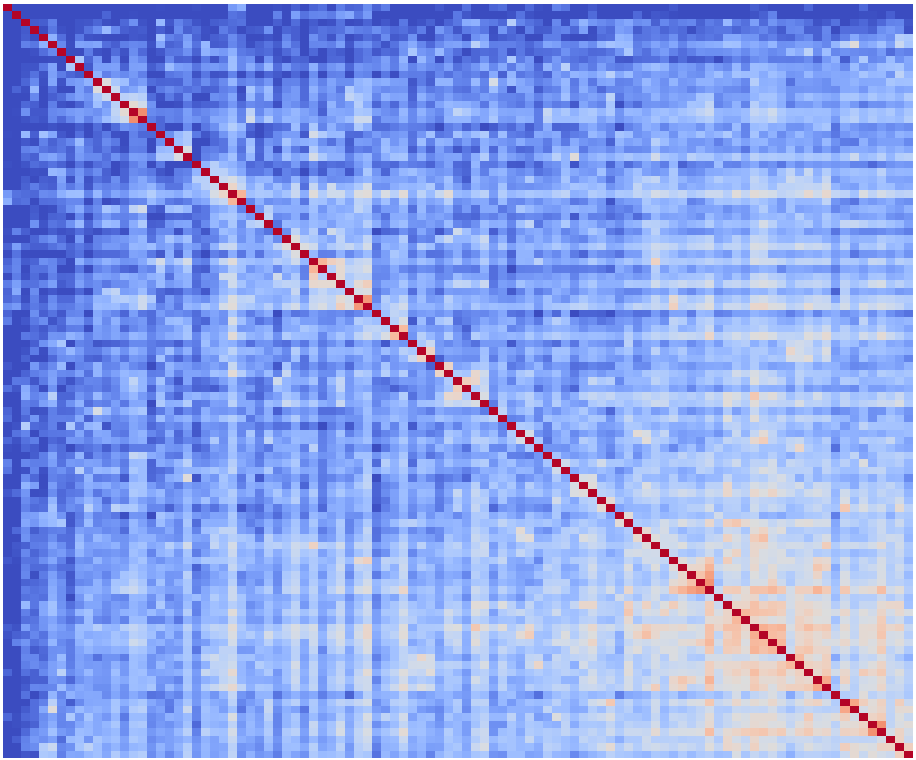}
        \caption{CaFo on \textit{Food101}}
        \label{fig:Food101cafo}
    \end{subfigure}        
    \hspace{0.001\linewidth} % 控制水平间隔
    \begin{subfigure}{0.22\linewidth}
        \centering
        \includegraphics[width=\linewidth, height=0.57\linewidth]{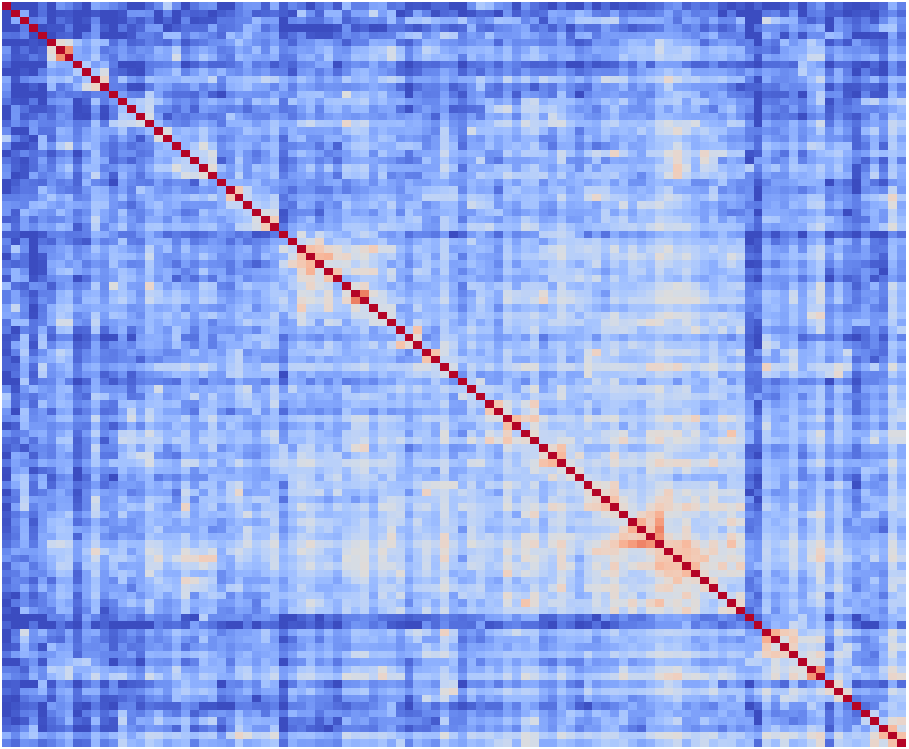}
        \caption{Sup on \textit{Food101}}
        \label{fig:Food101mine}
    \end{subfigure}    
    \hspace{0.001\linewidth} % 控制水平间隔
    \begin{subfigure}{0.22\linewidth}
        \centering
        \includegraphics[width=\linewidth, height=0.57\linewidth]{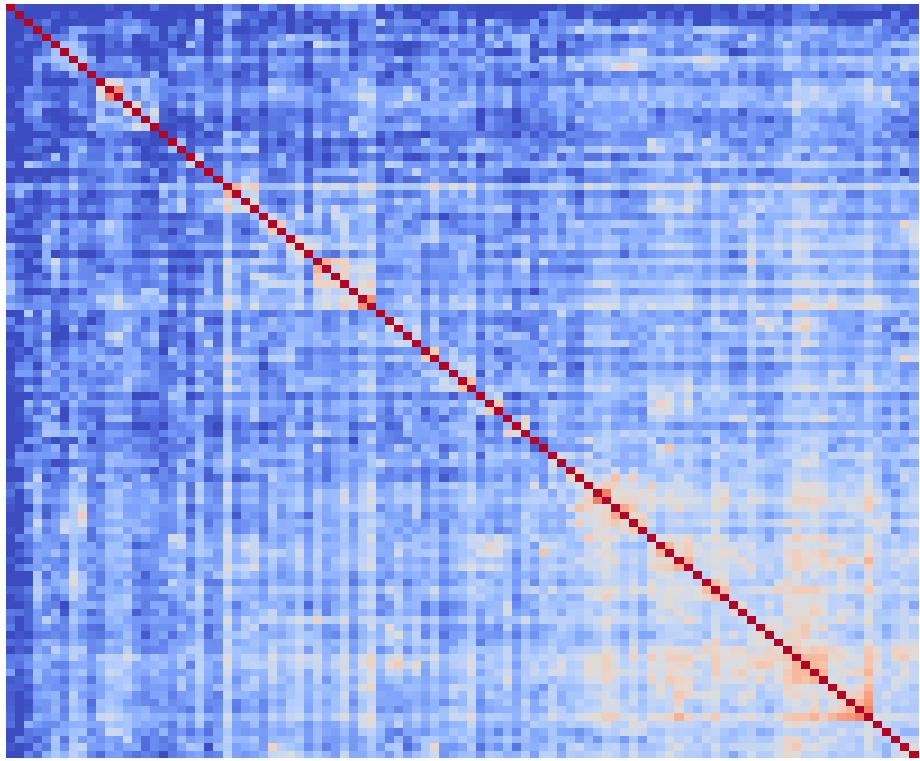}
        \caption{TPG on \textit{Food101}}
        \label{fig:Food101hunhe}
    \end{subfigure}

    \caption{Heatmap on the similarity among the category embeddings with different prompt descriptions on fine-grained image recognition tasks. All datasets have been used in the submission.
    % Org is the basic prompt, CaFo is prompt in \cite{Zhang_2023_CVPR}, Sup is supplement prompt, and TPG is the noimalization of Sup and CaFo. 
    }
    \label{fig:Heatmap1}
\end{figure*}

\begin{figure*}[htbp]
    \centering

    % \vspace{0.1cm} % 控制垂直间隔
    
    \begin{subfigure}{0.22\linewidth}
        \centering
        \includegraphics[width=\linewidth, height=0.57\linewidth]{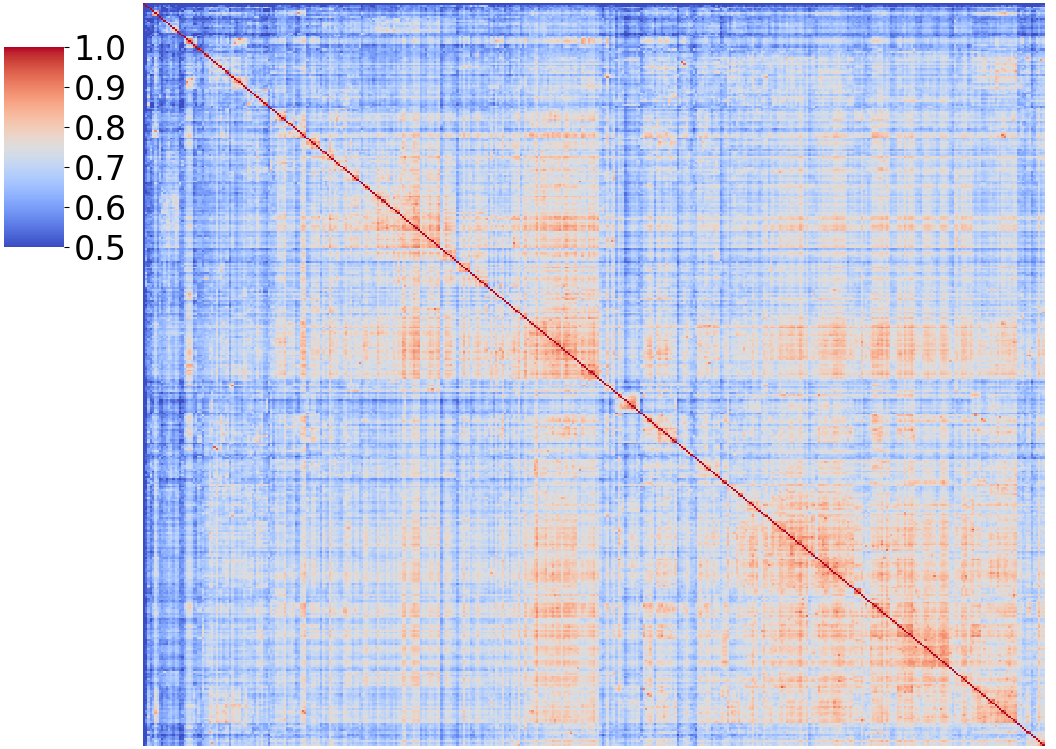}
        \caption{Org on \textit{SUN397}}
        \label{fig:SUN397org}
    \end{subfigure}
    \hspace{0.001\linewidth} % 控制水平间隔
    \begin{subfigure}{0.22\linewidth}
        \centering
        \includegraphics[width=\linewidth, height=0.57\linewidth]{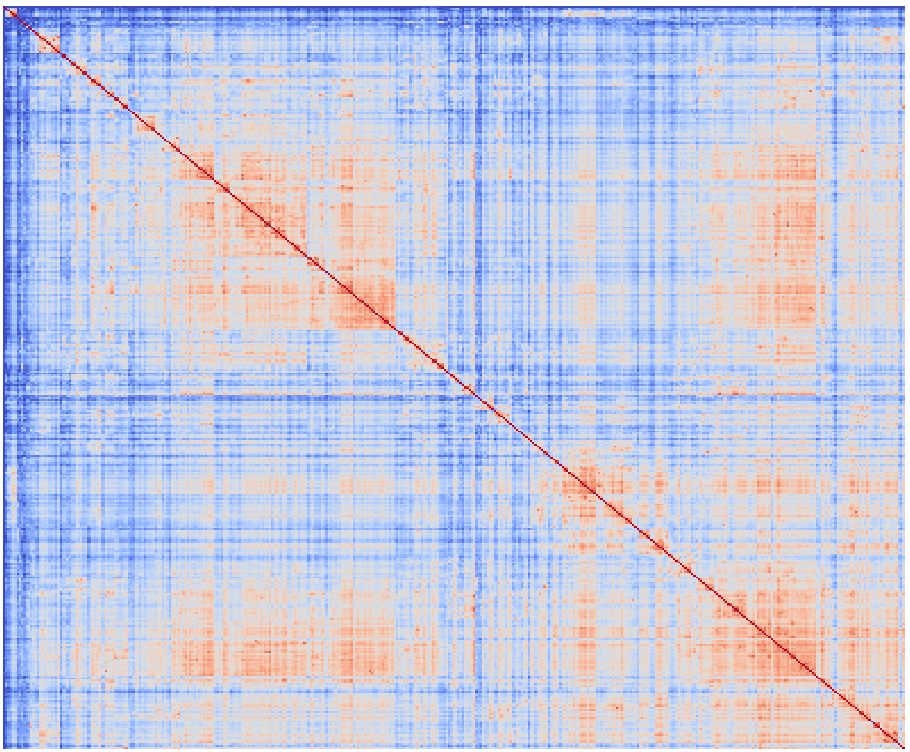}
        \caption{CaFo on \textit{SUN397}}
        \label{fig:SUN397cafo}
    \end{subfigure}        
    \hspace{0.001\linewidth} % 控制水平间隔
    \begin{subfigure}{0.22\linewidth}
        \centering
        \includegraphics[width=\linewidth, height=0.57\linewidth]{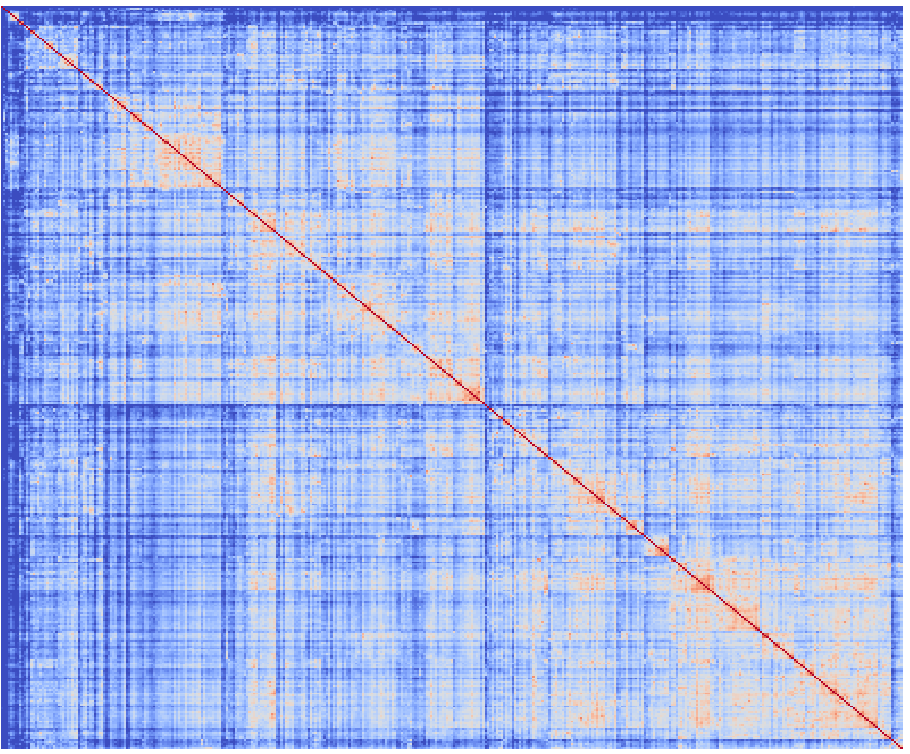}
        \caption{Sup on \textit{SUN397}}
        \label{fig:SUN397mine}
    \end{subfigure}    
    \hspace{0.001\linewidth} % 控制水平间隔
    \begin{subfigure}{0.22\linewidth}
        \centering
        \includegraphics[width=\linewidth, height=0.57\linewidth]{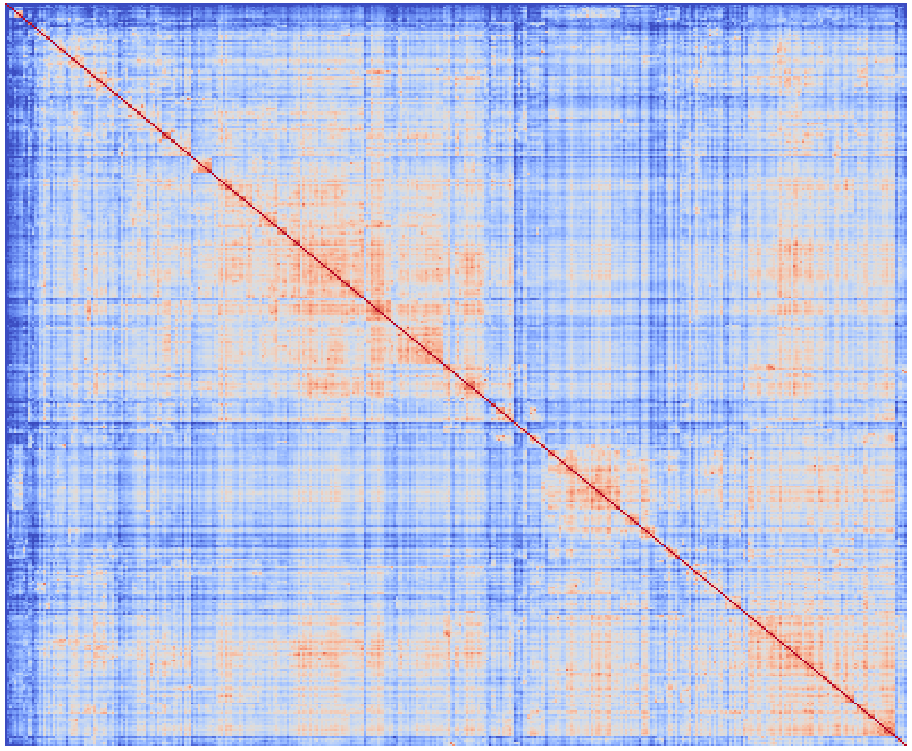}
        \caption{TPG on \textit{SUN397}}
        \label{fig:SUN397hunhe}
    \end{subfigure}

    % \vspace{0.1cm} % 控制垂直间隔

     \begin{subfigure}{0.22\linewidth} % 确保所有图的宽度相同
         \centering
         \includegraphics[width=\linewidth, height=0.57\linewidth]{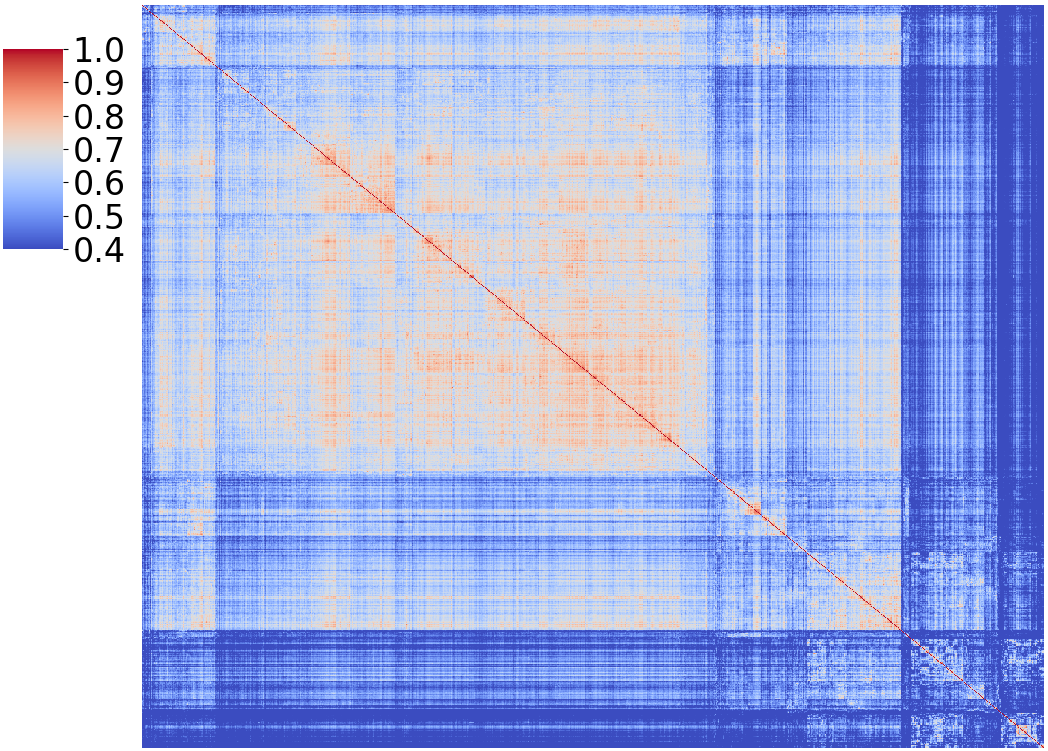}
         \caption{Org on \textit{Imagenet}}
         \label{fig:Imagenetorg}
     \end{subfigure}
     \hspace{0.001\linewidth} % 控制水平间隔
    \begin{subfigure}{0.22\linewidth}
        \centering
        \includegraphics[width=\linewidth, height=0.57\linewidth]{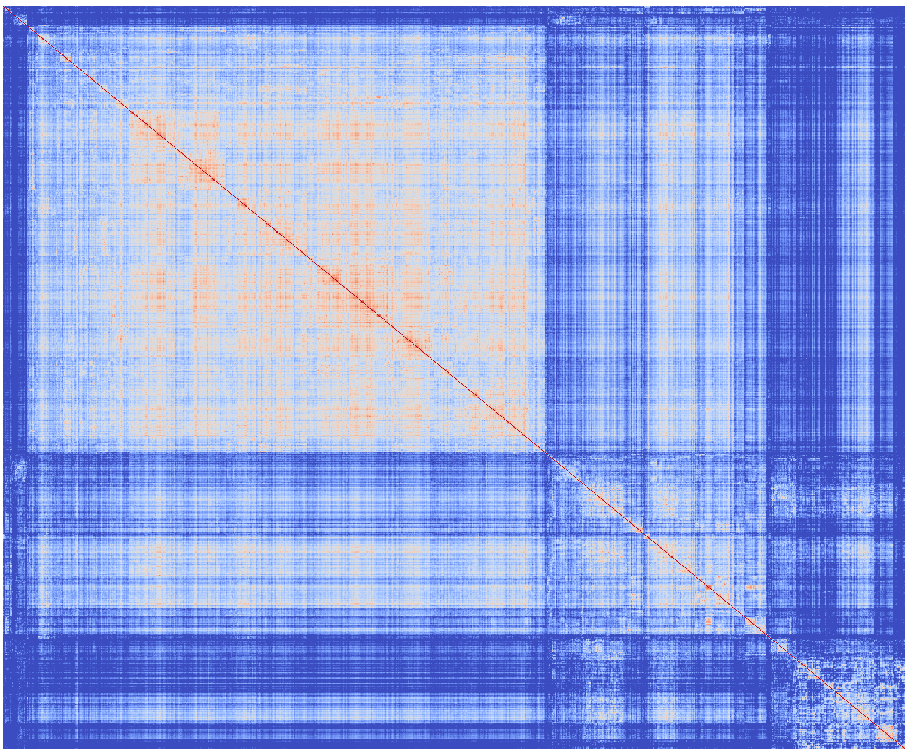}
        \caption{CaFo on \textit{Imagenet}}
        \label{fig:Imagenetcafo}
    \end{subfigure}
    \hspace{0.001\linewidth} % 控制水平间隔
    \begin{subfigure}{0.22\linewidth}
        \centering
        \includegraphics[width=\linewidth, height=0.57\linewidth]{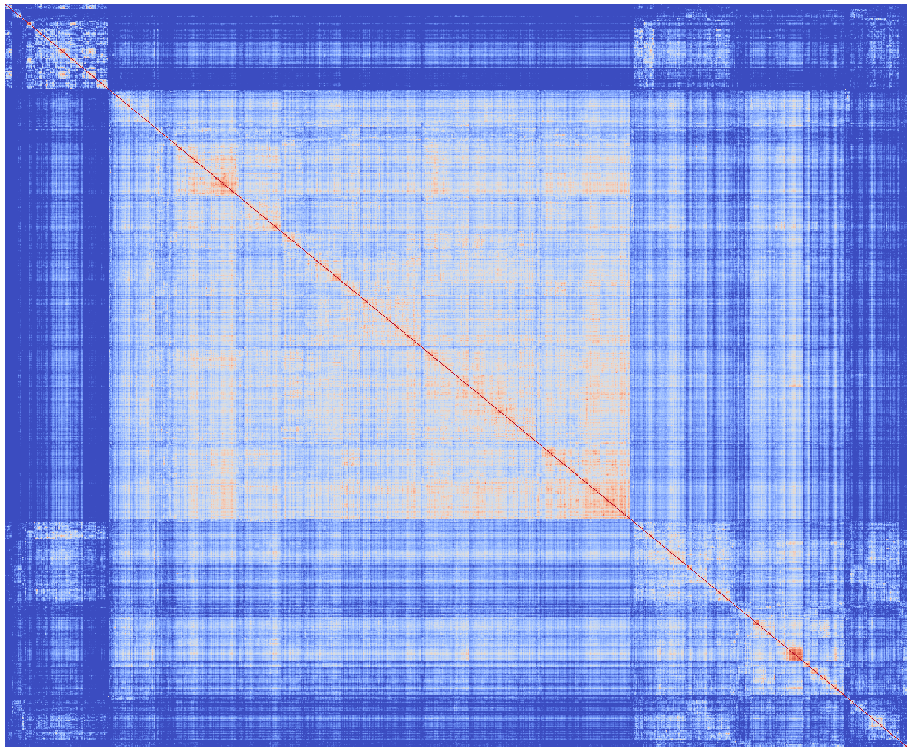}
        \caption{Sup on \textit{Imagenet}}
        \label{fig:Imagenetmine}
    \end{subfigure}    
    \hspace{0.001\linewidth} % 控制水平间隔
    \begin{subfigure}{0.22\linewidth}
        \centering
        \includegraphics[width=\linewidth, height=0.57\linewidth]{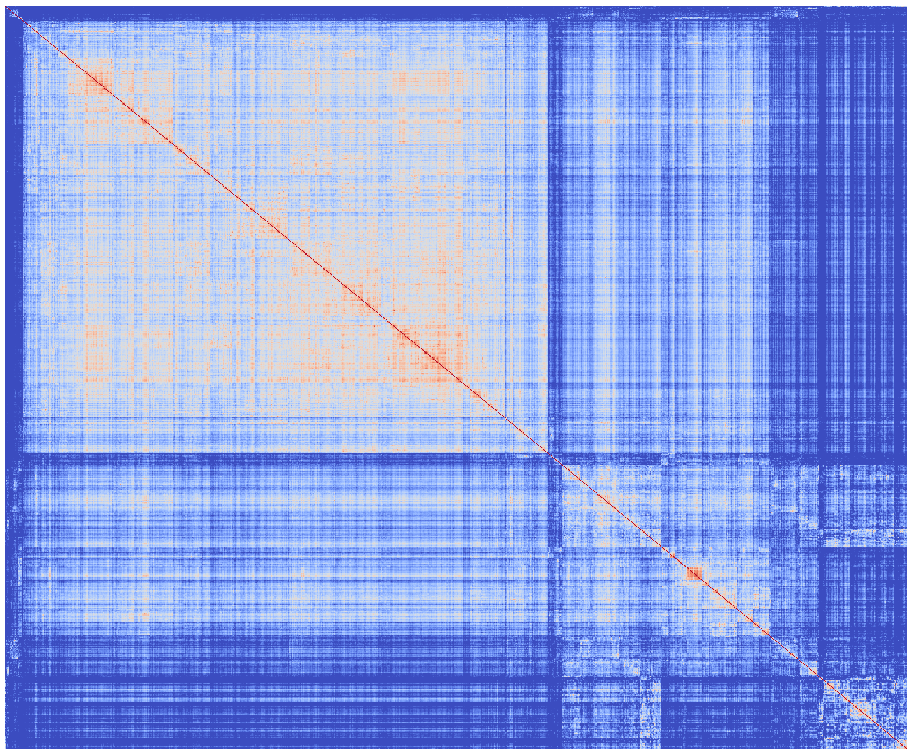}
        \caption{TPG on \textit{Imagenet}}
        \label{fig:Imagenethunhe}
    \end{subfigure}   
    
    % \vspace{0.1cm} % 控制垂直间隔

    \begin{subfigure}{0.22\linewidth}
        \centering
        \includegraphics[width=\linewidth, height=0.57\linewidth]{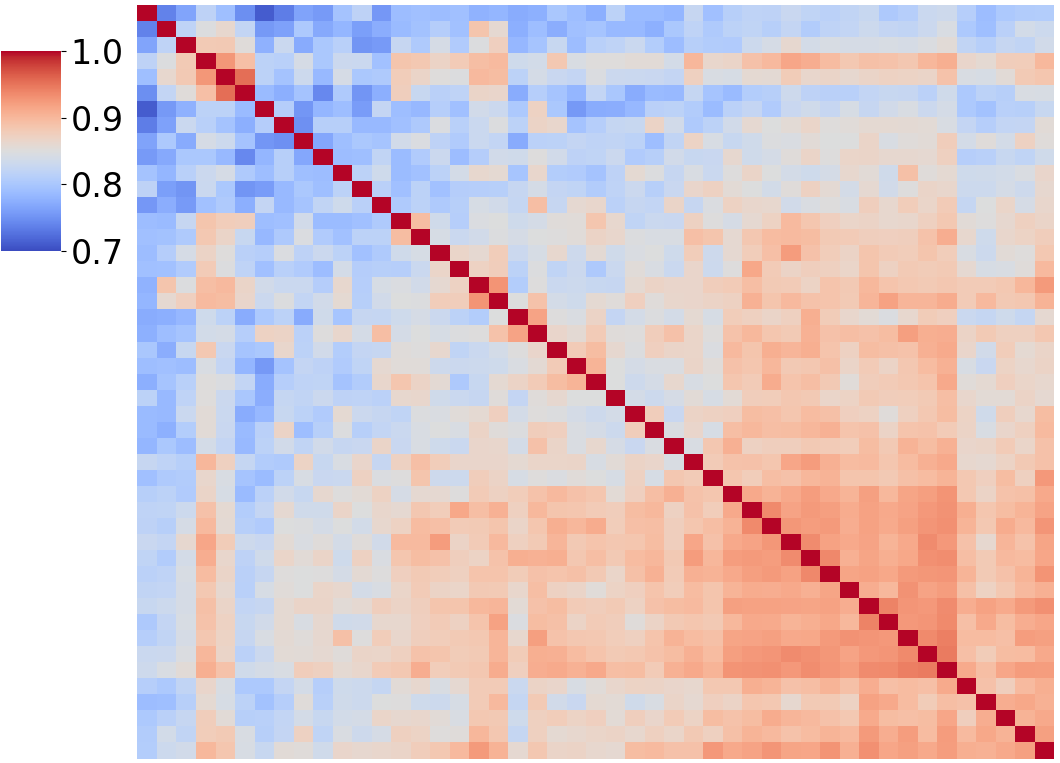}
        \caption{Org on \textit{DTD}}
        \label{fig:DTDorg}
    \end{subfigure}
    \hspace{0.001\linewidth} % 控制水平间隔
    \begin{subfigure}{0.22\linewidth}
        \centering
        \includegraphics[width=\linewidth, height=0.57\linewidth]{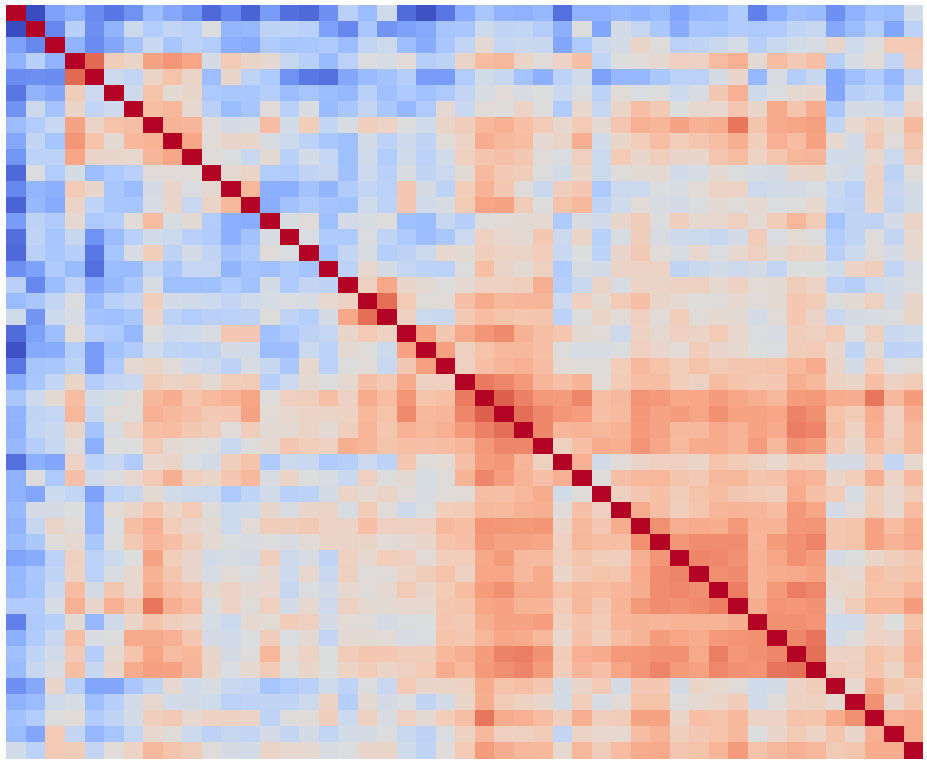}
        \caption{CaFo on \textit{DTD}}
        \label{fig:DTDcafo}
    \end{subfigure}        
    \hspace{0.001\linewidth} % 控制水平间隔
    \begin{subfigure}{0.22\linewidth}
        \centering
        \includegraphics[width=\linewidth, height=0.57\linewidth]{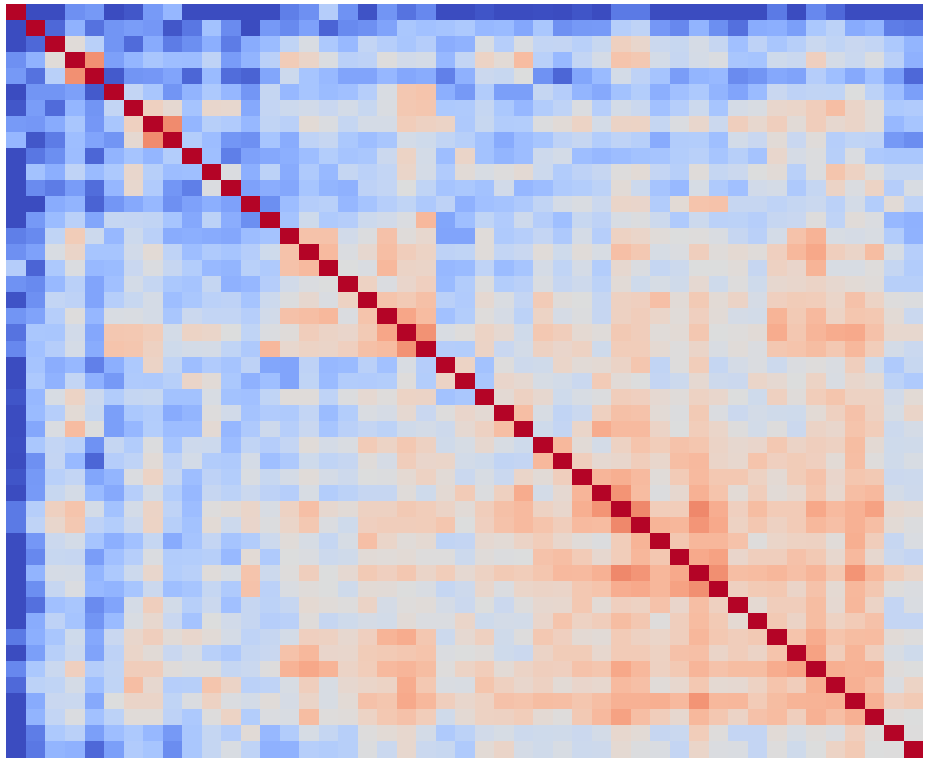}
        \caption{Sup on \textit{DTD}}
        \label{fig:DTDmine}
    \end{subfigure}    
    \hspace{0.001\linewidth} % 控制水平间隔
    \begin{subfigure}{0.22\linewidth}
        \centering
        \includegraphics[width=\linewidth, height=0.57\linewidth]{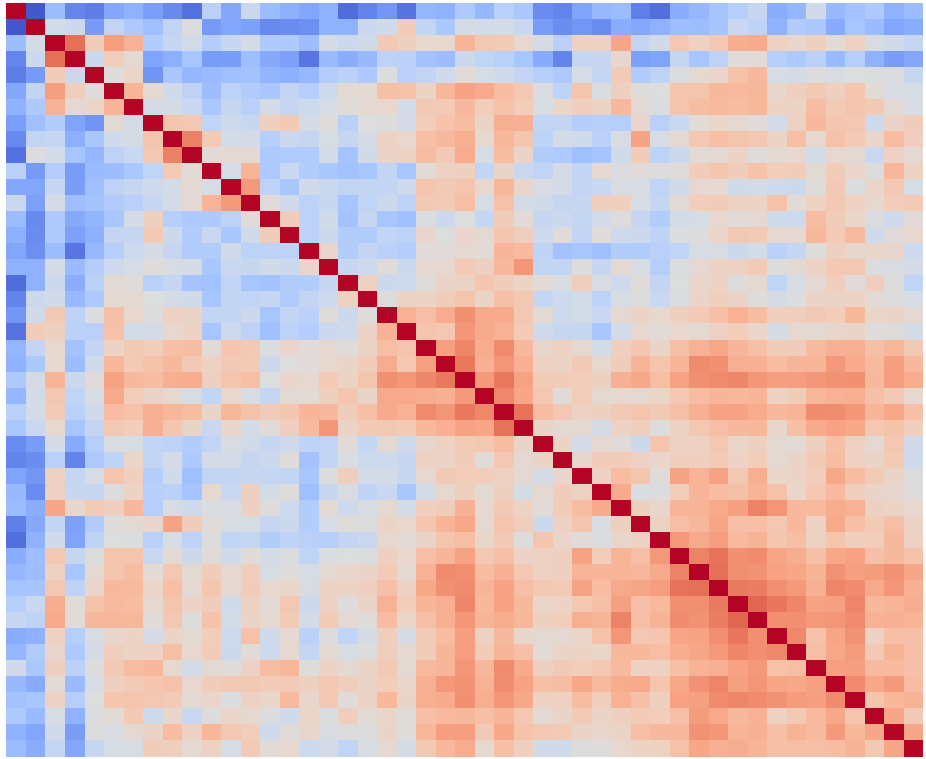}
        \caption{TPG on \textit{DTD}}
        \label{fig:DTDhunhe}
    \end{subfigure}

    \caption{Heatmap on the similarity among the category embeddings with different prompt descriptions on scene recognition task,  generic object recognition task and texture classification task respectively. All datasets have been used in the submission.}
    \label{fig:Heatmap2}
\end{figure*}

\begin{table*}[htbp]
    \centering
    \setlength{\tabcolsep}{1.3mm}
    \begin{tabular}{cccccccccccccccc}
        \toprule
        \multirow{2}{*}{Methods} & \multicolumn{5}{c}{\textit{Imagenet}} & \multicolumn{5}{c}{\textit{SUN397}} & \multicolumn{5}{c}{\textit{UCF101}} \\
        \cmidrule(lr){2-6} \cmidrule(lr){7-11} \cmidrule(lr){12-16}
         & 0 & 0.2 & 0.4 & 0.6 & 0.8 & 0 & 0.2 & 0.4 & 0.6 & 0.8 & 0 & 0.2 & 0.4 & 0.6 & 0.8 \\
        \midrule
        Org  & 62.95 & 61.57 & 59.67 & 58.14 & 55.60 & 66.56 & 64.87 & 61.31 & 58.93 & 54.25 & 73.43 & 66.88 & 63.65 & 60.96 & 52.42 \\
        CaFo & 63.10 & 61.99 & 60.72 & 59.61 & 57.58 & 67.83 & 66.21 & 63.39 & 61.43 & 57.21 & 73.75 & 67.80 & 65.13 & 62.52 & 53.40 \\
        Sup  & 61.61 & 60.11 & 58.79 & 57.32 & 55.00 & 66.79 & 65.18 & 61.46 & 59.56 & 55.14 & \textbf{74.94} & 68.20 & 64.84 & 61.80 & 55.62 \\
        TPG  & \textbf{63.21} & \textbf{62.11} & \textbf{60.84} & \textbf{59.84} & \textbf{57.70} & \textbf{68.65} & \textbf{66.58} & \textbf{63.61} & \textbf{62.02} & \textbf{58.17} & 74.73 & \textbf{68.73} & \textbf{67.12} & \textbf{63.18} & \textbf{55.93} \\
        \midrule
        \multirow{2}{*}{Methods} & \multicolumn{5}{c}{\textit{Caltech101}} & \multicolumn{5}{c}{\textit{StanfordCars}} & \multicolumn{5}{c}{\textit{Food101}} \\
        \cmidrule(lr){2-6} \cmidrule(lr){7-11} \cmidrule(lr){12-16}
         & 0 & 0.2 & 0.4 & 0.6 & 0.8 & 0 & 0.2 & 0.4 & 0.6 & 0.8 & 0 & 0.2 & 0.4 & 0.6 & 0.8 \\
        \midrule
        Org  & \textbf{91.81} & 90.43 & 90.18 & 88.32 & 82.39 & 69.22 & 58.71 & 53.40 & 49.20 & 39.57 & 78.27 & 78.19 & 77.60 & 77.38 & \textbf{69.33} \\
        CaFo & 91.28 & 90.47 & 89.61 & 88.15 & 81.70 & 69.26 & 60.02 & 54.47 & 50.23 & 40.46 & 78.46 & 78.37 & 77.29 & 76.98 & 68.93 \\
        Sup  & 91.60 & 90.34 & 89.66 & 87.95 & 83.29 & 69.17 & 58.97 & 54.57 & 48.63 & 37.77 & 77.67 & 77.97 & 76.72 & 76.85 & 69.18 \\
        TPG  & \textbf{91.81} & \textbf{90.59} & \textbf{90.22} & \textbf{88.88} & \textbf{83.94} & \textbf{69.64} & \textbf{60.09} & \textbf{56.10} & \textbf{50.86} & \textbf{39.96} & \textbf{78.97} & \textbf{78.99} & \textbf{77.95} & \textbf{77.98} & 68.75 \\
        \midrule
        \multirow{2}{*}{Methods} & \multicolumn{5}{c}{\textit{OxfordPets}} & \multicolumn{5}{c}{\textit{Flowers102}} & \multicolumn{5}{c}{\textit{DTD}} \\
        \cmidrule(lr){2-6} \cmidrule(lr){7-11} \cmidrule(lr){12-16}
         & 0 & 0.2 & 0.4 & 0.6 & 0.8 & 0 & 0.2 & 0.4 & 0.6 & 0.8 & 0 & 0.2 & 0.4 & 0.6 & 0.8 \\
        \midrule
        Org  & 87.14 & 86.86 & 83.32 & 75.90 & 58.16 & 92.45 & 84.21 & 76.21 & \textbf{65.12} & 54.69 & 64.36 & 57.09 & 50.53 & 43.90 & 42.67 \\
        CaFo & 88.01 & 87.14 & \textbf{83.76} & 76.56 & 59.58 & 92.16 & 84.21 & 74.38 & 64.31 & 55.99 & 65.37 & 58.10 & \textbf{53.72} & \textbf{51.24} & \textbf{48.40} \\
        Sup  & 87.82 & 86.43 & 82.56 & 76.37 & 58.19 & 91.88 & 84.65 & \textbf{77.22} & 64.31 & 54.85 & 64.48 & 55.61 & 50.41 & 45.39 & 40.25 \\
        TPG  & \textbf{88.58} & \textbf{87.38} & 83.54 & \textbf{77.05} & \textbf{59.63} & \textbf{92.57} & \textbf{85.87} & 76.90 & 63.82 & \textbf{56.76} & \textbf{65.90} & \textbf{58.16} & 53.25 & 49.70 & 47.22 \\
        \bottomrule
    \end{tabular}
    \caption{Accuracy (\%) with different prompts. All datasets have been used in the submission.}
    \label{tab:combinedalldata}
\end{table*}

\subsection{Accuracy With Different Prompts}

We test the performance of prompts with different noisy ratios to verify the prompt generalization on various datasets in \cref{tab:combinedalldata}, where all datasets are used in the submission manuscript.
We fine-tune the CLIP-Adapter with four different prompts and observe that our prompts perform well in general object detection, car, food, and scene understanding tasks. However, there are still some limitations in fine-grained tasks such as flower classification and texture discrimination.

TPG prompt achieves the highest accuracy in most noisy settings, even outperforming others on clean data.
As the noisy ratio increases, the accuracy reduction of TPG is minimal in these four prompts,
demonstrating its robustness to noisy data.
In addition, the better performance in the clean data proves that TPG effectively influences the similarity ranking in CLIP-Adapter.
Considering the similarity heatmap with the results in \cref{tab:combinedalldata},  Sup prompt is not helpful for recognition tasks with smaller similarities.
The reason is that Sup prompt disrupts the inherent relationship of the text-image matching knowledge from the CLIP.

\begin{figure*}[t]
    \centering
    \begin{subfigure}{0.9\linewidth}
        \centering
        \includegraphics[width=0.9\linewidth, height = 0.17\linewidth]{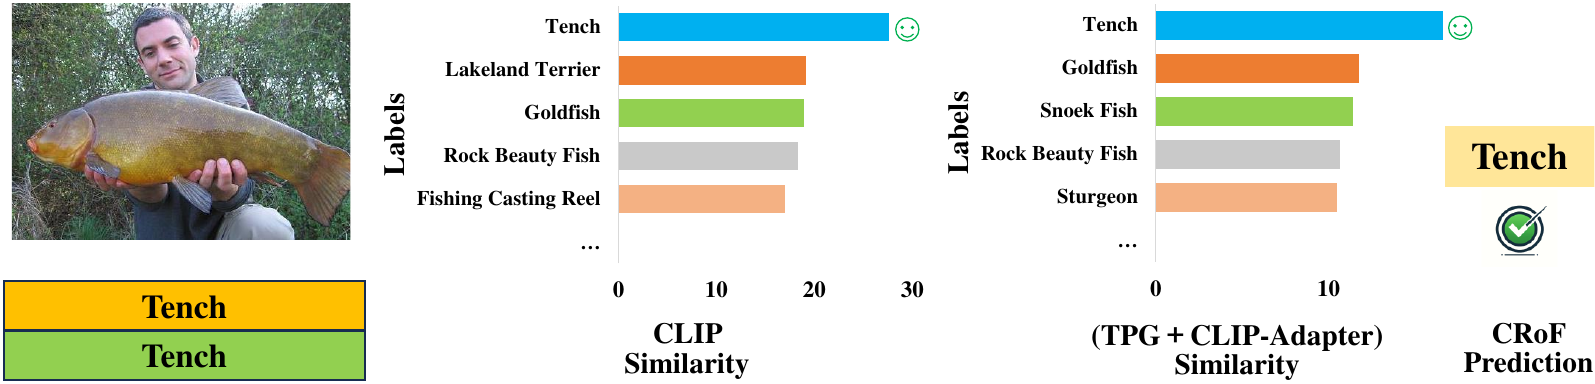}
        \caption{Both CLIP and (TPG+CLIP-Adapter) achieve correct matching.}
        \label{fig:duiduidui}
    \end{subfigure}
    
    \vspace{0.2cm} % 增加垂直间隔

    \begin{subfigure}{0.9\linewidth}
        \centering
        \includegraphics[width=0.9\linewidth, height = 0.17\linewidth]{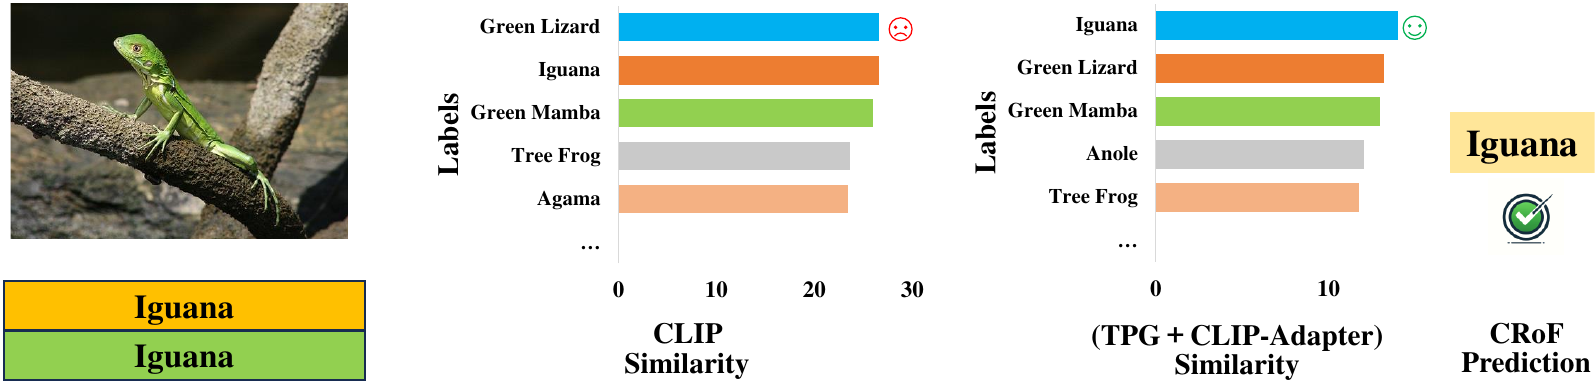}
        \caption{CLIP produces incorrect matching, while (TPG+CLIP-Adapter) achieves correct matching.}
        \label{fig:duicuodui}
    \end{subfigure}
    
    \vspace{0.2cm} % 增加垂直间隔

    \begin{subfigure}{0.9\linewidth}
        \centering
        \includegraphics[width=0.9\linewidth, height = 0.17\linewidth]{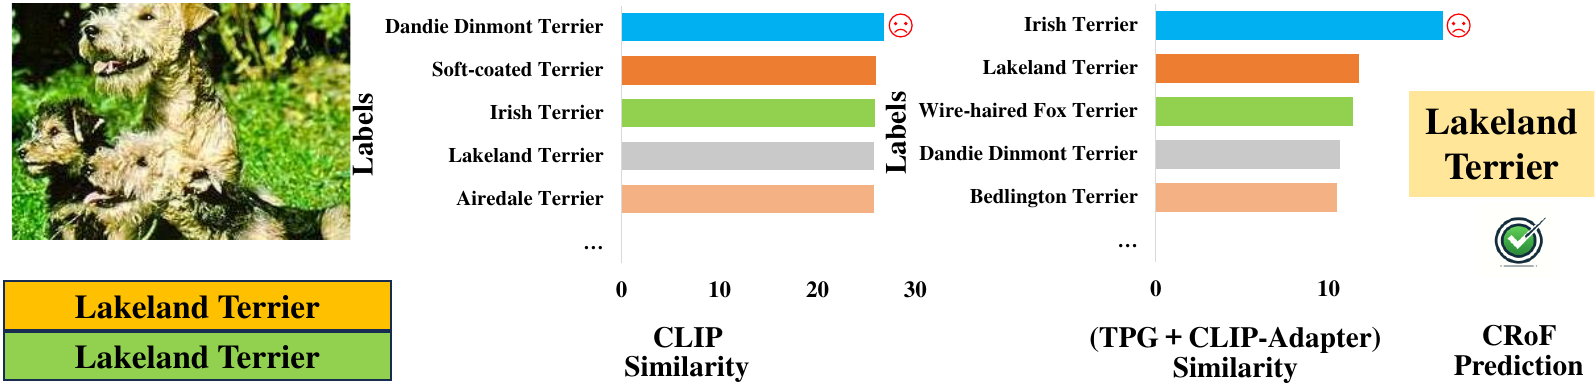}
        \caption{Both CLIP and (TPG+CLIP-Adapter) produce incorrect matching.}
        \label{fig:duicuocuo}
    \end{subfigure}
    
    \caption{Three visualized samples when an original label is ground truth.}
    \label{fig:keshihua1}
\end{figure*}

  \begin{figure*}[t]
    \centering
    \begin{subfigure}{0.9\linewidth}
        \centering
        \includegraphics[width=0.9\linewidth, height = 0.17\linewidth]{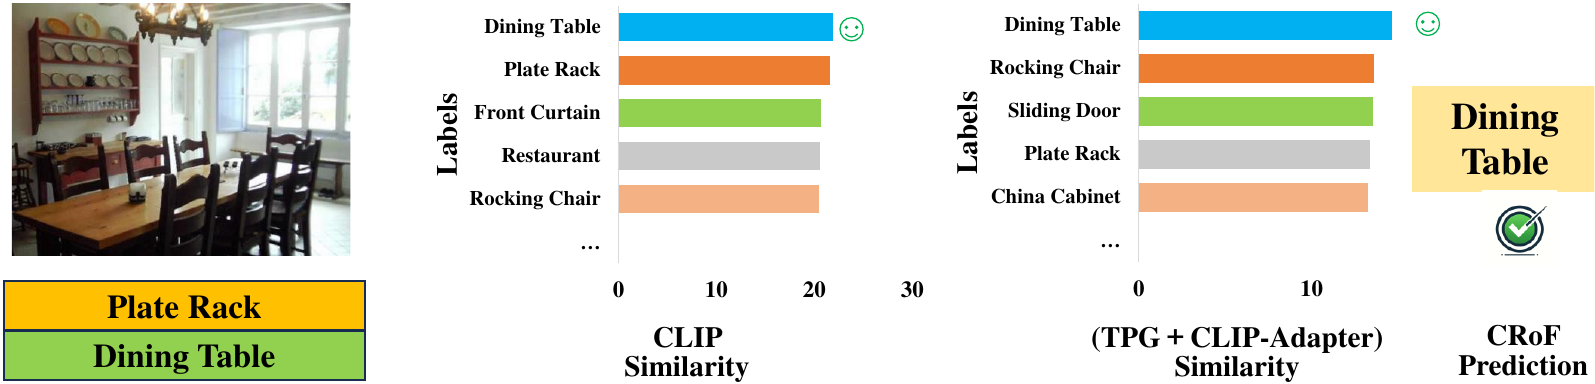}
        \caption{Both CLIP and (TPG+CLIP-Adapter) achieve correct matching.}
        \label{fig:cuoduidui}
    \end{subfigure}
    
    \vspace{0.2cm} % 增加垂直间隔

    \begin{subfigure}{0.9\linewidth}
        \centering
        \includegraphics[width=0.9\linewidth, height = 0.17\linewidth]{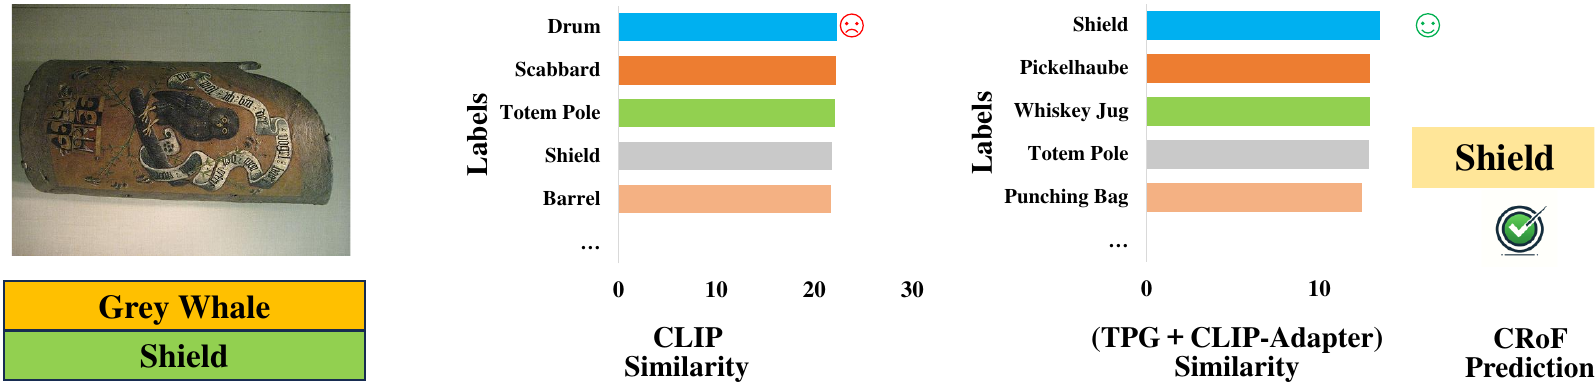}
        \caption{CLIP produces incorrect classifications, while (TPG+CLIP-Adapter) achieves correct matching.}
        \label{fig:cuocuodui}
    \end{subfigure}
    
    \vspace{0.2cm} % 增加垂直间隔

    \begin{subfigure}{0.9\linewidth}
        \centering
        \includegraphics[width=0.9\linewidth, height = 0.17\linewidth]{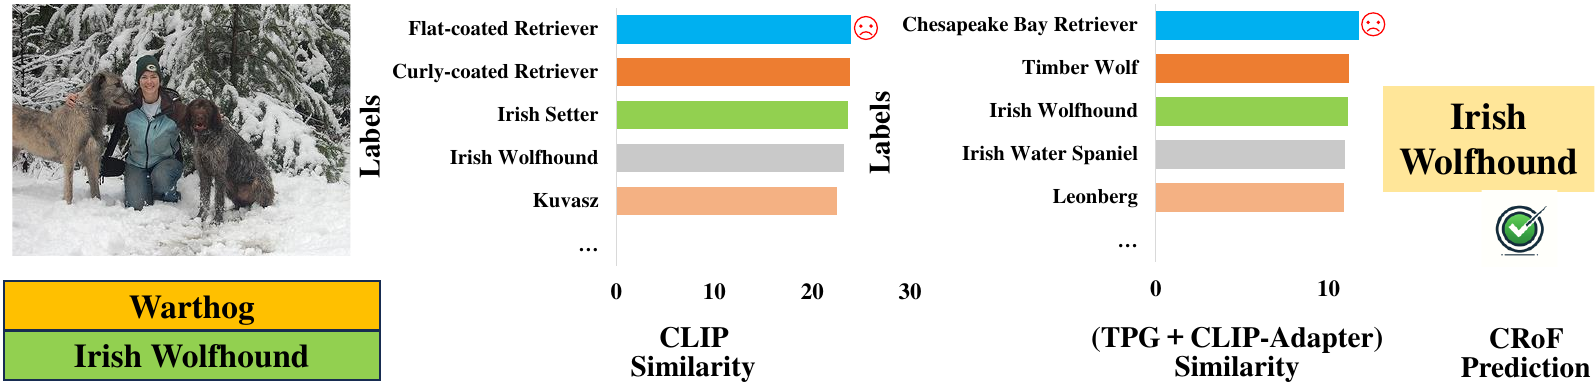}
        \caption{Both CLIP and (TPG+CLIP-Adapter) produce incorrect matching.}
        \label{fig:cuocuocuo}
    \end{subfigure}
    \caption{Three visualized samples when the original label is ground truth.}
    \label{fig:keshihua2}
 \end{figure*}
\section{Visualization}

 Our proposal CRoF, \textbf{C}LIP-based  \textbf{Ro}bust \textbf{F}ew-shot learning,  is effective in recognizing the target class with corrected similarity.
 We select several typical classification visualizations.
 All the experiments are conducted on the ImageNet dataset using a 10-shot setting with a noise ratio of 0.4
 The left column shows the images with their original label (highlighted in orange rectangle) and ground truth label (highlighted in green rectangle). 
 The two bar charts illustrate the similarity rank calculated by vanilla CLIP and our proposed methods.
CLIP in this figure represents the similarity ranking directly computed by the vanilla CLIP model. 
TPG+CLIP-Adapter refers to the combination of TPG prompt and CLIP-Adapter to enhance the accurate matching in similarity ranking. 
The right column shows the final classification results obtained by CRoF.
Depending on whether the original label is the ground truth or not, there are two scenarios as follows.

\subsection{Performance on Correct Original Label}
 As illustrated  in \cref{fig:keshihua1}, we select three groups of data with correct original labels (ground truth labels). 
 From \cref{fig:duiduidui}, it can be observed that when CLIP classifies correctly, our method (TPG+CLIP-Adapter) also gives the correct matching.  
 There is no doubt that CRoF achieves correct classification when the ground truth label is available. 
In \cref{fig:duicuodui}, although the original label is correct, vanilla CLIP leads to the mismatching with the noisy correspondence by recognizing  "\textit{Green Lizard}" as the most similar category, which causes confusion in the subsequent multiple label weighting module and affects the performance of our method. 
By employing (TPG+CLIP-Adapter), the correct category "\textit{Iguana}" ranks up as the most similar category.
\cref{fig:duicuocuo} illustrates a particularly challenging case.
The category "\textit{Lakeland Terrier}" has many similar categories in the ImageNet dataset, making mismatching easier. As a result, both CLIP and (TPG+CLIP-Adapter) initially predict incorrect labels with the highest similarity.
However, (TPG+CLIP-Adapter) ascends the correct category "\textit{Lakeland Terrier}" from CLIP’s fourth to  second position in the ranking. This adjustment enables the subsequent multiple label weighting module to receive accurate label information, allowing CRoF to achieve the correct classification result.

\subsection{Performance on Noisy Original Label}
We select three typical examples with incorrect original labels, as shown in \cref{fig:keshihua2}.
In \cref{fig:cuoduidui}, although both CLIP and (TPG+CLIP-Adapter) successfully identify the correct ground truth label "\textit{Dining Table}" as the most similar category, the noisy incorrect label "\textit{Plate Rack}" is a highly confusable category. 
Vanilla CLIP ranks it as the second most similar category, while (TPG+CLIP-Adapter) ranks it fourth. 
If the subsequent multiple label weighting module takes top-3 predictions, (TPG+CLIP-Adapter) significantly reduces misclassification caused by the wrong label.
In \cref{fig:cuocuodui}, for the image with ground truth "\textit{Shield},"  "\textit{Drum}" is matched as the most similar label in CLIP and  "\textit{Shield}" ranks fourth. 
This ranking prevents the correct label from giving a contribution effectively to the multiple label weighting.
However, (TPG+CLIP-Adapter) ranks the correct label first, ensuring accurate classification by CRoF.
\cref{fig:cuocuocuo} illustrates an extremely challenging situation with many highly confusable categories.
CLIP ranks the ground truth label "\textit{Irish Wolfhound}" fourth, whereas (TPG+CLIP-Adapter) ranks it in third position. 
This optimization ensures that the correct label information is effectively transferred to the multiple label weighting module, which helps increase accuracy.

% \section{Code Release} 
% For more implementation details of our CRoF, we provide the prompt and all the training processes on the $Caltech101$ dataset as an example in a zip file. It consists of an executable main function and relative classes.
